# Supplementary material for: Residential Demand Response Applications Using Batch Reinforcement Learning
Source: arXiv:1504.02125 source file (2015-04-08)
Supplement: Supplementary file 1 [file appendix.tex]

\appendices

\section{Model equations}
Here we describe the model equation of the electric water heater and climate control.

\subsubsection{Electric water heater}

\subsubsection{Climate control}
The transfer function of a household with heat pump is modeled using the following second-order Equivalent Thermal Parameter (ETP) model~\cite{chassin2008gridlab,Sonderegger}
\begin{equation}
\begin{matrix}
\dot{T}_{a} &=& \frac{1}{C_{a}} \left[T_{m}H_{m} - T_{a}\left(U_{a}+H_{m}\right)+Q_{a}+T_{o}U_{a}\right]\\
\dot{T}_{m} &=& \frac{1}{C_{m}}\left[H_{m}\left(T_{a}-T_{m}\right)+Q_{m}\right],
\end{matrix}
\label{eqTCL}
\end{equation}
where $Q_{a}$ and $Q_{m}$ are defined by
\begin{equation}
\begin{matrix}
Q_{a} &=& \alpha Q_{s} + \beta Q_{i} + Q_{hp}\\
Q_{m} &=& (1-\alpha) Q_{s} + (1-\beta)Q_{i}.
\end{matrix}
\end{equation}

%Here $U_{a}$ is the conductance of the building envelope, $T_{out}$ is the outside air temperature, $T_{in}$ is the inside air temperature, $T_{m}$ is the inner mass temperature, $H_{m}$ is the conductance between the inner air and the solid mass $C_{a}$ is the thermal mass of the air and $C_{m}$ is the thermal mass of the interior solid mass.
%The heat flux into the interior air mass $Q_{a}$ is given by a fraction $\alpha$ of the heat gains of the internal loads $Q_{i}$, a fraction $\beta$ of the solar heat gains $Q_{s}$ and the heat gain generated by the heat pump  $Q_{hp}$.
%The other fraction of $Q_{i}$ and $Q_{s}$ are added to the interior solid mass.

\begin{table} [h!]%
\caption{Equivalent Thermal Parameters for a house of 150 $m^2$}
    \label{ETP_parameters}
\begin{center}
\begin{tabular}{ l  c  c }
\toprule
 Parameters   & Low thermal integrity & High thermal integrity \\
   \midrule
    $U_{a} [W/{}^\circ C]$    &  1154 &  272    \\   
    $H_{m} [W/{}^\circ C]$    &  6863 &  6863   \\   
		$C_{a} [MJ/{}^\circ C]$   &  2,441 &  2,441 \\   
    $C_{m} [MJ/{}^\circ C]$   &  9,896 &  9,896 \\   
  \bottomrule
\end{tabular}
\end{center}      
\end{table}

\section{Cross-entropy parameters}
